# Supplementary material for: Training Language Models with Language Feedback
Source: arXiv:2204.14146 source file (2022-11-17)
Supplement: Supplementary file 1 [file old_appendix_tables.tex]

\clearpage
\onecolumn
\begin{table*}[h!]
\centering
\begin{tabular}{p{13.5cm}}
\hline
\textbf{\textit{Example 1}} \\
\hline
\\
\textbf{Original Summary} \\
Should the author ask her committed boyfriend if he lied about visiting an old flame? \\
\\
\textbf{Feedback} \\
The summary is good but should mention more details. Concretely, it should remove the word "committed", since that isn't emphasized in the text. The summary should also mention that the author believes her boyfriend visited an old flame very early on in their relationship, i.e. after 4 months. Further the summary should mention that her boyfriend has already denied that this happened when the author asked him when they were both drunk. It should also convey that the boyfriend has lied before. The author is asking if she should mention this issue or not, since it would bring peace but she already had brougth it up once. \\
\\
\hdashline
\\
\textbf{Feedback Refinement + Reranking} \\
The author is considering asking her boyfriend if he lied about visiting an old flame early on in their relationship, as this has been bothering her. He already denied it when asked drunk, and he has lied to her before. \\
\\
\textbf{Feedback Refinement} \\
The author is considering asking her boyfriend if he lied about visiting an old flame early on in their relationship, after he denied it when asked while drunk. She is worried about how this would add to the list of his past lies. \\
\\
\textbf{General Refinement} \\
The author is considering asking her committed boyfriend if he lied about visiting an old flame, and she is torn about whether or not to do so. \\
\\
\textbf{Human Reference Summary} \\
Asked my bf once if he went to go meet a girl, but i think he lied. Should I ask if he lied? \\
\\
\hline

\textbf{\textit{Example 2}} \\
\hline
\\
\textbf{Original Summary} \\
my boyfriend invited me to spend Mother's Day with his parents but I feel weird about it because I don't want to imply that I will become their daughter one day. Is this too soon or am I overthinking it? \\
\\
\textbf{Feedback} \\
The summary is mostly correct but it should mention that one of the reason why the original poster feels weird about all this situation is because their relationship is just starting and they haven't talked about a future together yet. It is also important that the original poster can't spend they Mother's day with her mom and this is one of the reasons why her boyfriend has invited her. \\
\\
\hdashline
\\
\textbf{Feedback Refinement + Reranking} \\
The original poster is feeling weird about spending Mother's Day with their boyfriend's parents because they haven't talked about a future together yet. They also can't spend Mother's Day with their own mom. \\
\\
\textbf{Feedback Refinement} \\
The original poster feels weird about spending Mother's day with their boyfriend's parents because they haven't talked about their relationship yet, but they should go because it will be a good opportunity to get to know them better. \\
\\
\textbf{General Refinement} \\
My boyfriend invited me to spend Mother's Day with his parents, but I feel weird about it because I don't want to imply that I will become their daughter one day. Is this too soon or am I overthinking it? \\
\\
\textbf{Human Reference Summary} \\
my boyfriend and I have been together 8 months and he invited me to spend Mother's Day with his mom and dad, but I feel uncomfortable too soon? \\
\\
\hline

\textbf{\textit{Example 3}} \\
\hline
\\
\textbf{Original Summary} \\
Girl (F/19) doesn't know what to do with guy (M/21) who is good and polite, but not romantic and doesn't want anything serious. \\
\\
\textbf{Feedback} \\
The summary should make clear that the girl is already together with the guy for 7 months. The summary should also point out that the guy is not passionate and doesn't want sex. Lastly the summary should convey that the author is frustrated by the fact that the guy doesn't want anything serious and says he doesn't want to go fast, but that she also thinks she's in love. \\
\\
\hdashline
\\
\textbf{Feedback Refinement + Reranking} \\
Girl (F/19) is dating guy (M/21) who is good and polite but not romantic and doesn't want anything serious. Girl is frustrated because she wants more than what the guy is willing to give. \\
\\
\textbf{Feedback Refinement} \\
Girl (F/19) is frustrated with guy (M/21) because he is good and polite, but not romantic and doesn't want anything serious. \\
\\
\textbf{General Refinement} \\
Girl (F/19) doesn't know what to do with guy (M/21) who is good and polite, but not romantic and doesn't want anything serious. \\
\\
\textbf{Human Reference Summary} \\
He (21) is a good guy, but I'm afraid he doesn't want anything serious with me (19).  How should I react? \\
\\
\hline

\textbf{\textit{Example 4}} \\
\hline
\\
\textbf{Original Summary} \\
Snipped my fingers, bled all over the kitchen, and then fell on my ass. Summary: Today, the author's seventh day working at a restaurant, the county mandated that they must wear gloves when handling food. \\
\\
\textbf{Feedback} \\
The first part of the summary is correct but the second one should not be there. Instead of mentioning that it was the seventh day of work, the summary should mention how the author fell twice after cutting the finger when trying to remove the tips of the mandatory gloves. \\
\\
\hdashline
\\
\textbf{Feedback Refinement + Reranking} \\
Today, the author cut their fingers while trying to remove the tips of gloves mandated by the county, and then fell twice. \\
\\
\textbf{Feedback Refinement} \\
The author cut their fingers, bled all over the kitchen, and then fell on their ass. \\
\\
\textbf{General Refinement} \\
The author cut their fingers, bled all over the kitchen, and then fell on their ass. \\
\\
\textbf{Human Reference Summary} \\
Attempted to make finger-less gloves with my hand in the glove, and fell twice on wet floors, which I had not done in the last 2 years. \\
\\
\hline

\textbf{\textit{Example 5}} \\
\hline
\\
\textbf{Original Summary} \\
A girl I know from high school is sending mixed messages about meeting up. I'm not sure what to do next. \\
\\
\textbf{Feedback} \\
The summary is good, but it should also point out that the woman is about to leave the country for a year. The author feels like she is attracted to him. The summary should also convey that the author is explicitly asking if he should ask her if she is actually interested or if he should just move on. \\
\\
\hdashline
\\
\textbf{Feedback Refinement + Reranking} \\
A girl I know from high school is sending mixed messages about meeting up. I'm not sure what to do next. The woman is about to leave the country for a year. \\
\\
\textbf{Feedback Refinement} \\
A girl I know from high school is sending mixed messages about meeting up. I'm not sure what to do next. \\
\\
\textbf{General Refinement} \\
A girl I know from high school is sending mixed messages about meeting up. I'm not sure what to do next. \\
\\
\textbf{Human Reference Summary} \\
Asked a girl out I've been texting for a while. Says she up for seeing me but her actions imply she doesn't actually want to. \\
\\
\hline

\textbf{\textit{Example 6}} \\
\hline
\\
\textbf{Original Summary} \\
Girl invites guy to church youth event, guy gets ignored and ditched by girl, guy is contemplating not going to the event anymore. \\
\\
\textbf{Feedback} \\
The summary is quite correct but misses some important points. The summary should mention that before the church youth event the original poster and the girl already had a wonderful time. It is also important that the author was upset because the girl was feely with another guy during the church youth. \\
\\
\hdashline
\\
\textbf{Feedback Refinement + Reranking} \\
The girl had a great time with the guy before the church youth event, but then she ignored him and was touchy-feely with another guy during the church youth event. The guy is contemplating not going to the event anymore. \\
\\
\textbf{Feedback Refinement} \\
The girl invited the guy to a church youth event, the guy got ignored and ditched by the girl, and the guy is contemplating not going to the event anymore. \\
\\
\textbf{General Refinement} \\
A girl invites a guy to a church youth event, but the guy gets ignored and ditched by the girl. The guy is now contemplating not going to the event anymore. \\
\\
\textbf{Human Reference Summary} \\
girl invites me to something she ditches me at; forgets I'm a human being at one point or another. \\
\\
\hline

\textbf{\textit{Example 7}} \\
\hline
\\
\textbf{Original Summary} \\
A woman is starting a strength training routine and wants opinions on her list of machines. \\
\\
\textbf{Feedback} \\
The summary is good, but should convey more details about the individuals situation. Concretely the individual is losing a lot of weight and now also wants to build muscles. The summary should also point out that the individual does not want to use free weights. \\
\\
\hdashline
\\
\textbf{Feedback Refinement + Reranking} \\
A woman is starting a strength training routine and is looking for opinions on her list of machines. She is losing weight and wants to make sure she builds muscle. She is not comfortable using free weights. \\
\\
\textbf{Feedback Refinement} \\
A woman is starting a strength training routine and wants opinions on her list of machines. She is losing weight and does not want to use free weights. \\
\\
\textbf{General Refinement} \\
A woman is starting a strength training routine and wants opinions on her list of machines. \\
\\
\textbf{Human Reference Summary} \\
I think I should use the above machines to target all of my muscle groups. Please let me know if I left something out and what MACHINE, if any, I can use to target that muscle/group. \\
\\
\hline

\textbf{\textit{Example 8}} \\
\hline
\\
\textbf{Original Summary} \\
My boyfriend cheated on me two years ago and now he wants to be friends with the girl he cheated on me with. I'm not sure if I'm ready for that. \\
\\
\textbf{Feedback} \\
The summary is quite accurate but it does not mention that the original poster's boyfriend was in love with the girl with whom he cheated her and that the original poster thinks that he still loves her. \\
\\
\hdashline
\\
\textbf{Feedback Refinement + Reranking} \\
The original poster's boyfriend cheated on her two years ago and now he wants to be friends with the girl he cheated on her with. The original poster is not sure if she is ready for that. \\
\\
\textbf{Feedback Refinement} \\
The original poster's boyfriend cheated on her two years ago and now he wants to be friends with the girl he cheated on her with. The original poster is not sure if she is ready for that. \\
\\
\textbf{General Refinement} \\
My boyfriend cheated on me two years ago and now he wants to be friends with the girl he cheated on me with. \\
\\
\textbf{Human Reference Summary} \\
Boyfreind cheated was okay with it. but now he wants to talk to her they were good freinds so i dont feel okay saying no. but im really not okay with it yet \\
\\
\hline

\textbf{\textit{Example 9}} \\
\hline
\\
\textbf{Original Summary} \\
The writer is considering breaking up with their long-term girlfriend, citing their increased confidence and changed perspective since the two were last together. They are worried about the potential implications of breaking up, but are unsure of what to do. \\
\\
\textbf{Feedback} \\
The summary is not correct. The summary should mention that the authors girlfriend broke up twice with him and cheated on him during that period. The summary also has to mention that the author is now thinking about breaking up because he wants to live the single life and have fun with other women. The author wants advice on what to do, since he loves his girlfriend also very much and wants to be together with her in the long run. \\
\\
\hdashline
\\
\textbf{Feedback Refinement + Reranking} \\
The author is considering breaking up with their long-term girlfriend because they want to date other people and have fun. The girlfriend has cheated on the author in the past, and the author is worried about the potential implications of breaking up. \\
\\
\textbf{Feedback Refinement} \\
The author is considering breaking up with their long-term girlfriend because they have evolved and want to experience more of life. \\
\\
\textbf{General Refinement} \\
The writer is considering breaking up with their long-term girlfriend, citing their increased confidence and changed perspective since the two were last together. They are worried about the potential implications of breaking up, but are unsure of what to do. \\
\\
\textbf{Human Reference Summary} \\
My gf cheated on me years ago, I wish I had that opportunity.  Want to have my cake and eat it too. \\
\\
\hline

\textbf{\textit{Example 10}} \\
\hline
\\
\textbf{Original Summary} \\
Girlfriend is skeptical about long-distance relationship working, needs some positive encouragement. \\
\\
\textbf{Feedback} \\
This summary is good overall, but it should mention that original poster's boyfriend is dedicated to the relationship even if the worries coming from the girl are getting him down. \\
\\
\hdashline
\\
\textbf{Feedback Refinement + Reranking} \\
Girlfriend is worried about long-distance relationship, needs some positive encouragement. Boyfriend is dedicated to the relationship, even if worries from girlfriend are getting him down. \\
\\
\textbf{Feedback Refinement} \\
Girlfriend is worried about long-distance relationship, needs some positive encouragement. Boyfriend is dedicated to the relationship, but worries are getting him down. \\
\\
\textbf{General Refinement} \\
Girlfriend's boyfriend has gotten a job in the US, and they're worried about their long-distance relationship. They're looking for some positive stories about long-distance relationships that have worked out well. \\
\\
\textbf{Human Reference Summary} \\
Boyfriend moving abroad for work in a couple of months. I'm terrified that things won't work out. I've only heard the bad stories. Should I have faith and trust it will be okay? \\
\\
\hline

\end{tabular}
\caption{Examples of summaries, human-written feedback, and generated refinements.}
\label{tab:example_summaries}
\end{table*}
\clearpage
\twocolumn
